# Supplementary material for: Automatic and Structure-Aware Sparsification of Hybrid Neural ODEs
Source: arXiv:2505.18996 source file (2026-03-03)
Supplement: Supplementary file 1 [file Re-fitting.tex]

\textbf{Optional Re-fitting to Enforce Exact Sparsity}
%Due to a number of design and optimization choices, such as choosing $\lambda$ with cross-validation, 
In minimizing the proposed non-convex loss with a $L_1$ penalty,  %being non-differentiable at 0, using 
many out-of-the-shelf-optimizer-based SGD may shrink weights for redundant edges to very small values but not necessarily exactly zero. Even with this numerical issue resolved, weights of some redundant edges still tend be non-zero with $\lambda$ selected via CV optimizing the predictive performance. %often do not get shrunk to 0 exactly, but to very small values near 0. 
%Such practical sparsity is often sufficient for the purpose of reducing model variance and improving predicitve performance, since edges with small weights contribute negligibly to predictions and can be treated as "effectively zero" for practical purposes. However, 
In cases where exact sparsity is desired (for example, for the sake of interpretability) or the bias introduced by the regularization is deemed too high, an optional post-LASSO re-fitting step can be helpful. %In our own experiments, 
%Since re-fitting may not have a significant impact on prediction performance, it is optional. 
%but does introduce extra computational cost, so we make it optional and leave it to readers.

To implement the re-fitting step, note that we perform a $K$-fold CV in identifying the optimal set of hyper-parameters for the optimization problem in (\ref{eq:loss}) denoted by $(\lambda_1^*, \lambda_2^*).$ 
Let $(\Theta_k^*,W_k^*, \beta_k^*)$ be the resulting minimizer based on 
$D^{(-k)},$ the training data with the $k$th part from the CV removed.
To stabilize weights estimation,  we take the average of $K$ sets of estimated weights obtained from different data splits,$W^*=K^{-1}\sum_{k=1}^K W^*_k,$ as the final weights. 
Then, we select a positive empirical threshold $w_0$ and perform edge selection by keeping only edges whose estimated weights' magnitudes are higher than $w_0$, i.e., edge $(u, v)\in E^{a, c}$ is removed if $|w^*_{(u,v)}|\le w_0.$ Once, we have obtained the reduced graph, denoted by $\widetilde{G}^{a, c},$ we then re-train MNODE with a new loss function 
 $$   \sum_{\text{cases}, h}\left\|S_{\text{obs}}^{a,t_h}-\hat{S}_{\text{obs}}^{a,t_h}\left(\hat{S}^{a,t_0}(\cdot; \beta),\cdot ; \Theta, \mathbf{1},\widetilde{G}^{a,c} \right)\right\|_2^2+\lambda_3\|\Theta\|_2^2$$
where the hyperparameter $\lambda_3$ can be selected via a fresh $K$-fold CV. %The resulting 
To adaptively choose the threshold $w_0$, one can introduce a noise input node directly connected to all observable states in step 1:
\begin{equation*}
    \begin{split}
        V^{a, c} &\leftarrow V^{a, c}\cup \{ x_{\varepsilon}\};\\
        E^{a, c} &\leftarrow E^{a, c} \cup \{(x_{\varepsilon}, s)\mid s \in S_{\text{obs}}^a\},
    \end{split}
\end{equation*}
and then set the threshold to be the the maximum edge weight associated with the noise input $x_\varepsilon$ in $W^*$:
\[w_0=\max_{s\in S_{\text{obs}}^a} |w^*_{(x_\varepsilon,s)}|,\]
i.e., the selected empirical threshold can effectively filter out this known noise node.
