# Supplementary material for: Automatic and Structure-Aware Sparsification of Hybrid Neural ODEs
Source: arXiv:2505.18996 source file (2026-03-03)
Supplement: Supplementary file 3 [file rebuttal.tex]

\section*{Rebuttal Draft}



\subsection{Reviewer 1}

\begin{itemize}
\item {\bf Model class expressiveness: Does the proposed sparsification framework assume linearity in the mechanistic model parameters? If so, how does this limit applicability to nonlinear systems common in healthcare and other fields? }

We did not impose any specific functional form for the mechanistic model and our method can be used to simplify general nonlinear mechanistic models.

\item {\bf Generalization to larger mechanistic graphs: How does performance scale with increasing state dimensionality or interaction complexity? Any expected limitations? }

First, our framework imposes no restrictions on interactions between states. Second, as demonstrated in our synthetic experiment comparing reduced versus comprehensive starting graphs, the benefit of our method becomes more pronounced when the initial graph is large and contains redundant edges. In our current work, we focus on biomedical applications, where clinically validated mechanistic models rarely involve more than 50 states because constructing and validating substantially larger models is extremely challenging in practice.

We agree that extending the approach to massive graphs with hundreds or thousands of states is conceptually appealing. Based on our limited experience, such generalization appears feasible, and the associated computational burden should increase approximately linearly with the number of states. Exploring applications in domains where high-dimensional mechanistic models are common represents an important future research direction. Additional methodological developments—such as knockoff-based procedures—may be required to enable valid inference on the sparsified model.

\item {\bf Practical deployment: What guidance can you provide for practitioners on choosing sparsity regularization strengths and graph-modification thresholds?}

We use standard cross-validation to choose these hyper-parameters.

\item {\bf Training efficiency: Can you quantify computational savings (e.g., reduced training time, memory use) achieved through the learned sparsity?} 

Reduction methods: HGS, NS, EGL, EN all take about 2 hour to complete one repetition, Greedy and Random searches take about 24 hours. Reduced model: HGS reduced model takes only about 1 hour to complete training, while the full unreduced model takes about 2 hours. While these computation time would depend on the hardware environment, the relative saving of the our proposal is expected to be reproducible. 

\item {\bf Interpretability: Are there examples where the discovered reduced model aligns with clinical or mechanistic knowledge? If so, including brief commentary would strengthen the healthcare relevance.}

%Our learned structure also yields biologically plausible and novel insights (taken form Neurips rebuttal):

In our real-data example, the method eliminates edges associated with glucagon feedback, consistent with the well-established observation that individuals with T1D exhibit impaired glucagon responses during hypoglycemia (Hypoglycemia and Diabetes: A Report of a Workgroup of the American Diabetes Association and The Endocrine Society, Seaquist et al., 2011). Our findings further suggest that this suppression persists even during exercise-induced hypoglycemia—a novel hypothesis that may warrant future investigation.

In addition, the learned graph prunes intermediate compartments linking insulin and glucose, effectively identifying a shorter regulatory pathway. This result aligns with empirical evidence that insulin sensitivity increases during and after exercise, producing a more rapid glucose response (A systematic review and meta-analysis of exercise interventions in adults with type 1 diabetes, Yardley et al., 2014).

{\color{blue} Bob has added a short/refined version of the above to the end of experiment section}
\end{itemize}


\subsection{Reviewer 2}
\begin{itemize}
\item{\bf rationale of step 1 says that transforming the original graph into and RDAG reveals essential causal structure. What is the evidence for this? It also says that this improves training stability. Has this been shown in the experiments? What is the reason for this improvement in stability? How do self-loops allow more flexible modeling of intra-component dynamics? It is said to be a key principle of hybrid modeling (line 190), but I am unsure how this is established.}

A clean causal interpretation does not permit statements such as A causes B and B causes A simultaneously. Therefore, it is standard practice to transform graphs containing cycles into DAGs or restricted DAGs (RDAGs) to explore plausible causal structures. By treating each cycle as a single unit within the model, the resulting DAG yields an interpretable and simplified causal representation that preserves the essential elements of the original mechanistic system.

In addition, ODE systems and neural ODEs whose dependency graphs contain cycles are susceptible to three major sources of instability: blow-ups, exploding gradients, and stiffness. While blow-ups and exploding gradients are familiar concepts in the machine-learning community, stiffness is less commonly discussed. Nonetheless, stiffness is a critical property of ODE systems because stiff neural ODEs can be extremely unstable and difficult to solve numerically. Please see references  \url{https://pubs.aip.org/aip/cha/article-abstract/31/9/093122/1077547/Stiff-neural-ordinary-differential-equations} \url{https://www.sciencedirect.com/science/article/pii/S2950550X25000263}.

The following two examples are added to the appendix to illustrate these instabilities in a two-stage system with cycles. 
\begin{enumerate}
\item Consider a simple 2 state system with a circular dependence:
\begin{align*}
    &\frac{ds_1(t)}{dt}=as_1(t)+bs_2(t)\\
    &\frac{ds_2(t)}{dt}=cs_1(t)+ds_2(t).
\end{align*}
Let $\lambda_1$ and $\lambda_2$ be the eigenvalues of the Jacobian of the system, 
$$J=\begin{bmatrix} a & b\\ c& d\end{bmatrix}.$$ 
If $\lambda_i$ has a positive real part, then $|h\lambda_i+1|>1$ and the system is instable in that if one solves the ODE system with forward Euler method with a step size $h,$  then the update
\[S(t+kh)=\left(hJ+I\right)^kS(t)\]
blow up as $k$ increases. The two eigenvalues of $J$ are
\[\frac{1}{2}\left(a+d\pm\sqrt{(a-d)^2+4bc}\right).\]
If $bc> \max(ad, 0)$,  a eigen value has a positive real part and the system is instable. On the other hand, suppose the system is acyclic except for self-loops, say $ds_1(t)/dt$ depends on $s_2(t)$ but $ds_2(t)/dt$ does not depend on $s_1(t)$, then the eigen values of the upper triangular $J$
\[J=\begin{bmatrix} a & b \\ 0 & d\end{bmatrix}\]
are simply $a$ and $d$.  In such a case, this system is allowed to freely chose $b$ to model how $s_2(t)$ affects $ds_1(t)/dt$ without concerns of explosion, as long as $\max(a, d)<0$.  Similarly, when we discretize the ODE system and solve it with RNNs, then the gradient will also behave like: $\left(J+I\right)^k,$ which will cause the RNNs to have exploding gradients as $k$ increases. In summary, in the presence of cycles, there are more constraints on model parameters to ensure the stability of the system.


\item Second, consider the following dissipative version of the 2-state system with a circular dependence to illustrate the system stiffness \citep{kim2021stiff, worsham2025guide}:
\begin{align*}
    &\frac{ds_1(t)}{dt}=-s_1(t)+bs_2(t)\\
    &\frac{ds_2(t)}{dt}=~~cs_1(t)-~~s_2(t),
\end{align*}
with eigenvalues $-1\pm\sqrt{bc}$. Suppose that we have controlled for blowing up, e.g., $0<bc<1.$ The system stiffness is defined as the ratio between the magnitude of the fastest to slowest stable rates:
\[\kappa \equiv \frac{1+\sqrt{bc}}{1-\sqrt{bc}}.\]
Thus, $\kappa$ may still go to infinity, when $\sqrt{bc}\uparrow 1.$
On he other hand, without circular dependence (i.e., $c=0$,) these two eigenvalues are both $-1$ and the stiffness is a constant regardless of the value of $b$ and $c.$ Again there are more constraints to avoid the system stiffness in the presence of cycles.

\end{enumerate}

%With cycles the eigenvalues of the Jacobian depend on all entry values and are challenging to control stiffness/explosion/gradient norm all at the same time. Without cycles, the Jacobian will be upper triangular after rearrangement whose eigenvalues are simply diagonal elements, allowing the system to freely model off-diagonal elements without stability concerns.
 %   \item Two examples are provided in the appendix to illustrate blow-ups, exploding gradients and stiffness concepts in 2-state system.
 

By collapsing cycles into super-nodes, we reduce the risk of system instability by relaxing the constraints placed on the model parameters. To preserve the postulated dynamics within each collapsed cycle, we incorporate a self-loop with a flexible neural network at the corresponding super-node, compensating for the structural simplification.

Finally, our ablation study also confirms the benefits of this approach: the full HGS model consistently outperforms the version without Step 1 in both predictive accuracy and robustness.

%    \item The key principle, as stated in the pioneering work of PINN, by Raissi, Perdikaris and Karniadakis, is that NNs can approximate solutions to dynamical systems very well.


{\color{blue} Bob has re-written the rationale of step 1 in the main text to be more precise about what we mean and also added two toy examples in Appendix \ref{app:stability} to support the claim.}
    
%\end{enumerate}



\item {\bf The formulation of step 2 is too formal which leads to a decrease in clarity of the paper. It would be useful to start from intuition and build from there. For instance, it would be useful to first describe what is the intuitive description of a partial closure.}

An intuitive example of {\bf transitive closure} would be student's high school journey. Typically, one has to start from grade 9, followed by grade 10, 11 and finally grade 12. A transitive closure of {\em this journey} adds all possible ``grade skip" options while maintaining the reachability condition that one can only move from a lower grade to a higher one. So the transitive closure gives the student the option to jump from grade 9 right to grades 11 and 12 or jump from grade 10 to 12. 

The {\bf partial transitive closure} is a more conservative transitive closure in which the student is allowed to skip, but not right from the beginning to the end (i.e. immediately from 9 to 12). 

The rationale is %that many such intermediate latent states exist in physiological models to model delays (a student needs time to reach the level of grade 12), however, just like there are students we learn quickly and skip grades, there is also a lot of variability in how many delay states are need across individuals, and therefore, we want 
to provide the model all options in traveling a path, which would then be regularized and selected in final step. Without this step, every student would have to gradually move from grade 9 to 12. %, which may not be optimal. 
In the same time, we, however, do not want to be too aggressive in providing short-cuts. The partial closure would exclude the most aggressive path (a direct jump from 9 to 12), so that 
%if there is no such a path in the mechanistic prior (the school thinks that 
the student need to spend at least one intermediate year.

{\color{blue} Bob has modified the rational of step 2 paragraph to include this intuition}

\item {\bf The introduction to the paper claims that the method allows incorporating domain knowledge reduction of the graph. As far as I can tell in steps 1 and 2, the graph reduction methods are more structural (not data-driven) rather than incorporating domain knowledge.} 

Thanks for the constructive comment. In the original paper, we have tailored our algorithm to general biomedical domains by suggesting (1) all cycles should be removed (because in physiology, feedback loops are prevalent and are not as indispensable as in physical systems); (2) all short-cuts are permissible except those bypassing all latent states (because physiological models rarely model the response directly as a function of input);  and (3) all edges should be regularized (because there is often no strong clinical evidence about the necessity of particular edges).  In the revision, we have clarified that those are general suggestions for biomedical applications and are not rigid rules: users can still input their domain knowledge at specific applications by 
(1) setting up the mechanistic prior; (2) selecting cycles to be collapsed; 
(3) selecting short-cuts to be added; and (4) selecting edges to be kept (i.e.,  not regularized in step 3). 


\begin{comment}
\begin{enumerate}
    \item Acknowledge that there are two ways to interpret "domain-knowledge informed," and our method does allow both (but we did not make it very explicit in the paper)
    \item User-side domain knowledge: users can input their domain knowledge at
    \begin{enumerate}
        \item the mechanistic prior step
        \item step 1 selecting which cycles should be collapsed
        \item step 2 selecting which short-cuts should be added and which should not
        \item step 3 deciding which inputs should be regularizaed upon, and which ones should be kept and not penalized
    \end{enumerate}
    We have added a few sentences to our methodology section to emphasize the customizability.
    \item Algorithm designer-side domain knowledge: for the sake of general applicability and given ICLR is a general ML vanue, we authors, have implicitly make choices that we believe are most applicable to general biomedical domains:
    \begin{enumerate}
        \item at step 1, we implicitly assume that all cycles should be removed (because because in physiology, and in particular glycemic response, feedback loops are prevalent and at the same time, they are not as indispensable as in physical systems, and many such loops achieve equilibrium very fast  or can be approximated by a periodic function of time.
        \item at step 2, we decide that all short-cuts are permissible except ones allow inputs to bypass all latent states, because physiological models, while differing in number of latent states, rarely model the response directly as a function of input without latent dynamics.
        \item at step 3, we decide that all edges should be regularized because there isn't currently strong clinical evidence about the necessity of a particular edge.
    \end{enumerate}
    \item {\color{blue} Bob has added a customization paragraph to each step to emphasize this}
\end{enumerate}
\end{comment}


\item{\bf line 167. “maximally strongly” should be maximal strongly … There appears to be a formatting problem where line spacing has changed starting from page 5.}

{\color{blue} Bob: this has been corrected} Thanks for pointing this out, we have edited the word for MSCC. For the line spacing, we did not make modifications to the template or in the source file, it seems to be an artifact of the template itself adjusting line spacing adaptively.

\end{itemize}

\subsection{Reviewer 3}

\begin{itemize}
\item {\bf I’m a little confused by the motivation of the setup. In most instances I’m familiar with, the incentive for parameterizing a causal model or a dynamical system with a graph is interpretability, but the authors insist that the setup isn’t identifiable and the purpose is only for predicting future states. In that case, what is the rationale for insisting on DAG / RDAG structure at all? One could still encode prior knowledge by constraining dependence of one state variable on others with masking.}

Thanks for raising this important question. The interpretability is indeed important and is an advantage of a mechanistic model. We stated explicitly in intro and related work that our method has better interpretability than black-box methods. The reduced mechanistic model can be used for hypothesis generating and used for prediction purpose. Our caution of non-identifiability is about the risk of   causally interpreting of the original or reduced graph of the mechanistic model. Specifically, one should not consider a directional edge in the graph suggests that the value in one state determines the value in another state. Such a causal relationship requires validation from randomized experiments to perturb related states while controlling all potential confounders.  {\color{blue} Bob has modify section 2.5 to reflect this, we may also include a paragraph to discuss mechanistic interpretations of our results.}

Moreover, graph formalism provides a convenient and rigorous way to articulate our proposed modification to the original mechanistic model. Without terminologies such as maximal strongly connected components and transitive closures, it would be very cumbersome to rigorously define intuitive notions of ``circular dependence'' ($v_1 \rightarrow v_2 \cdots \rightarrow v_K \rightarrow v_1$) and ``short-cuts'' ($v_1 \rightarrow v_2 \rightarrow v_3 \Rightarrow v_1 \rightarrow v_3$). It also allows one to use out-of-shelf graph algorithms to implement step 1 and step 2 modifications rather than manually adding/masking states.


\item {\bf The third part of the model seems to just be the inclusion of L1/L2 regularization, which I think is straightforward enough to not be a novel portion of the proposed method.}

 We agree that the regularization idea is very natural and non-surprising. However, unlike well established regularizations such as L2 or L1 on the NN parameters, we believe that our proposal of coupling L1 regularization on edge specific weights with L2 regularization on neural network parameters is the first in ML community.  We have established the connection of this hybrid L1/L2 regularization with the conventional group LASSO penalty on the NN parameters. The new formulation is more general than the group lasso regularization and allows an efficient optimization algorithm. Therefore, we consider this proposal a novel contribution to the field. 



\item {\bf The highly varying y-axes across graphs makes it much much harder to gauge which performance improvements are substantial and which ones are almost negligible. I would suggest the authors use tables in some cases so a reader can more easily tell. For example, many bar plots in Figure 2b are somewhat misleading because the scale is so small.}

Thanks for pointing this out. It is indeed difficult to gauge the performance improvement, as scale and mangutitude of these metrics are highly domain and data dependent.  To address your concern, we provided a table version of the results in the appendix for interested reader, while keeping the Figures as a simple visualization of the presence or absence of difference in performance between different methods.  {\color{blue} Bob will include a table version of the results in the appendix for interested readers to refer to}.



\item {\bf To my understanding, only the MNODE based methods are given the prior graph determining the underlying dynamics? In that case it seems the comparisons to the black box NODE models are somewhat uninformative, without encoding that prior into the model (even as a form of regularization).}

You are right that the black-box models don't incorporate any prior domain knowledge. The hope is that observe data will eventually ``teach'' the black-box model on all relevant relationships between states. As another reviewer, readers may be interested in quantifying the potential gain of including an imperfect mechanistic prior in improving the prediction performance.  As shown by our synthetic experiments, it is not true that having a mechanistic prior will always be better than the black-box model, as the mechanistic prior, which in medicine is often reasonably good but not as accurate as in physics, may miss important relationship and restrict the prediction model. 


\end{itemize}

\subsection{Reviewer 4}
\begin{itemize}

\item {\bf My primary concern is how the model handles patient variability. The T1DEXI dataset includes 105 different people, and it's a physiological fact that glucose dynamics differ significantly between individuals. From my reading of Equation 1, the MNODE learns a single set of dynamics for everyone, i.e., an "average patient" model. This seems to sidestep an important challenge in this domain. Could you clarify if this is indeed the case, and if so, explain the rationale behind this choice? To be clear, this has been discussed extensively in recent years ([1-4] for example).}



Lastly, our method can be used to train the prediction model for individual patient if there is sufficient number of instances (data) for the specific patient of interest. In our applications, we have a large number of patients but only a few instances per patient, so can't train different prediction models for different patients. In clinical practice, the prediction model will often be used to make prediction for new patients. In such a case, prediction models specifically trained for existing patients (even if feasible) would not be useful. On the other hand, our prediction model is trained to optimize the average performance in a population and should have a good prediction accuracy for new patients from the same population. 

First, we want to emphasize that our proposed model is also tailored for individual patient in the sense that the initial values of relevant latent states of the individual is determined from the 4-hour history of that patient via an encoder. Those instance-specific initial values contribute to the final prediction.  

{\color{red} In the revision, we suggests a possible extension of the proposal to also train individual specific neural networks by treating our proposed model as a foundation model, if one is interested in making repeated predictions for the same individual.} 

{\color{blue} Bob has modified equation (1) to more explicitly reflect instance-dependency of the initial condition}
    


\item {\bf The paper mentions that the cross validation splits were created from a ``random permutation'' of the 342 time series. To avoid data leakage, it's standard practice in clinical ML to split data at the patient level (i.e., all data from a single person stays in one fold). Could you confirm whether your evaluation followed this practice? If not, the reported performance might not accurately reflect generalization to new, unseen patients.}

Thanks for the insightful comments.  We are aware of the risk of data leakage in evaluating the model performance.  However, our particular application is special:  it is well recognized that intra-patient variability can be as high as inter-patient variability among diabetic patients.  Therefore, predicting new cases of an existing patient is as hard as new patients. Please see references \url{https://ieeexplore.ieee.org/document/7587866}, \url{https://pmc.ncbi.nlm.nih.gov/articles/PMC8620341} and \url{https://www.sciencedirect.com/science/article/abs/pii/S1746809413001031}.
In our dataset, the average intra-patient and inter-patient variabilities of average glucose level are 54.24 and 55.10, respectively, also supporting the aforementioned claim.

%average glucose value recorded in instance $i$ and $s_i$ be the standard deviation of the glucose values recorded in instance $i$, let 
%    \[N_{\text{inter}}=\{(i,j)|i<j, \text{instance i and j are not from same patient}\} \]
%    \[N_{\text{intra}}=\{(i,j)|i<j, \text{instance i and j are from same patient}\} \]
%    Intra-patient glucose root-mean-squared difference in mean:
%    \[\sqrt{\frac{1}{|N_{\text{inter}}|}\sum_{(i,j)\in N_{\text{inter}}}(e_i-e_j)^2}=54.24\]
%    Inter-patient glucose root-mean-squared difference in mean:
%    \[\sqrt{\frac{1}{|N_{\text{intra}}|}\sum_{(i,j)\in N_{\text{intra}}}(e_i-e_j)^2}=55.10\]
%    Intra-patient glucose root-mean-squared difference in standard deviation:
%    \[\sqrt{\frac{1}{|N_{\text{inter}}|}\sum_{(i,j)\in N_{\text{inter}}}(v_i-v_j)^2}=22.75\]
%    Inter-patient glucose root-mean-squared difference in standard deviation:
%    \[\sqrt{\frac{1}{|N_{\text{intra}}|}\sum_{(i,j)\in N_{\text{intra}}}(v_i-v_j)^2}=22.67\]
       
Another important reason that we didn't conduct patient-level cross-validation is that we expect to deploy the model on both existing patients and new patients in practice. Thus, the model performance needs to evaluated on new cases of existing patients as well as on new patients. Splitting at patient level would overlook the former.  

{\color{blue} Bob has included a sentence in experiment section (page 8) and an extra paragraph in appendix to highlight this}
    


\item {\bf The paper uses the term MNODE, but it seems that the functional forms of the UVA-Padova model are discarded, with only the graph structure being retained. The actual dynamics are then learned by MLPs. This is a very weak form of mechanistic prior. It would be helpful to discuss the trade-offs here.}

Your observation is correct that the functional forms of UVA-Padova model are not used in the current proposal. However, several versions of hybrid modeling utilizing the functional forms are possible:
\begin{enumerate}
\item keep the functional form and only tune the NN for the initial conditions and model parameter $\beta$ in
        \[\frac{ds(t)}{dt}=f_m\left(s(t),t;\beta\right) ~\mbox{ and } s(0)=NN(z)\]
        \item keep functional form and add an NN to learn residuals:
        \[\frac{ds(t)}{dt}=f_m(s(t),t; \beta)+NN(s(t),t)\]
        \item completely discard the functional form:
        \[\frac{ds(t)}{dt}=NN(s(t), t)\]
    \end{enumerate}
Those approach has examined in our previous work.  There are trade-offs between different options. In general
\begin{enumerate}
\item More mechanistic prior--more mechanistic constraint on model space, require less training data, less likely to overfit, but less capable of learning complex/unknown dynamics not captured by the prior. 
\item More black-box--less constraint on model space, more flexible and capable of learning new dynamics/complex patterns, but more prone to over-fitting and require more training data to learn a good model.
\end{enumerate}
 For a more comprehensive discussion of hybrid modelling approach, please see \citet{zou2024hybrid}. 
{\color{blue} Bob has added a paragraph to related work to discuss general hybrid modeling techniques and trade-offs}



\item {\bf
It's worth noting that in the synthetic experiments, the TCN model starts to outperform HGS on the RMSE metric as the sample size grows to N=1000. While HGS remains more robust in terms of Peak RMSE, this suggests that its strong inductive bias might become a disadvantage when more data is available. Could you comment on this trade-off?}

Thanks for the insightful comments. Indeed, while informative, the mechanistic prior is never perfect.  While it brings down the variance, it also may induce systematic bias.  When sufficient data are available for training, the role of bias would dominate that of the variance in determining the predictive performance, and black-box models may be superior as our simulation study demonstrated.

{\color{blue} In the revision, we have included a comments on this trade-off.}
  
\end{itemize}
